# Supplementary material for: Toward Optimized VR/AR Ergonomics: Modeling and Predicting User Neck Muscle Contraction
Source: arXiv:2308.14841 source file (2023-08-28)
Supplement: Supplementary file 1 [file supplementary.tex]

\section{Obtaining Muscle Contraction Levels from Multi-Channel Raw EMG Signals}
\label{supplementary:emg-processing}

Following standard electromyography (EMG) signal processing approaches~\cite{sommerich2000use,reaz2006techniques}, we processed and transformed our collected multi-channel raw EMG signals (2D data) into overall neck muscle contraction levels (1D data), or \activationShort for short. \Cref{fig:emg-processing-pseudo-code} details our EMG data processing pipeline. In addition, each user's total \activationShort was linearly normalized to $[0, 1]$ to incorporate and mitigate muscular strength/morphology variations across users, such that the \activationShort values from different users are comparable/consistent and that machine learning on several users' combined data is feasible.

\begin{figure}[h!]
\begin{tcolorbox}[
    enhanced,
    attach boxed title to top left={xshift=6mm,yshift=-3mm},
    colback=moonstoneblue!20,
    colframe=moonstoneblue,
    colbacktitle=moonstoneblue,
    title=EMG to \activationShort Data Processing Pipeline,
    fonttitle=\bfseries\color{black},
    boxed title style={size=small,colframe=moonstoneblue},
    sharp corners]
\medskip
\begin{algorithmic}[1]
    \Function{EMG2\activationShort}{EMG}
        \State {\color{blue}\(\triangleright\) 4-channel EMG signals}
        \State $t = \Call{GetTimestamps}{\textsc{EMG}}$ {\color{blue} \Comment{EMG timestamps}}
        \State $\textsc{axis} = $ 0
        \State $\textsc{bandpass\_freq\_low} = $ 20 Hz
        \State $\textsc{bandpass\_freq\_high} = $ 150 Hz
        \State $\textsc{lowpass\_freq} = $ 1 Hz
        \State $\textsc{butterworth\_order} = $ 4
        \State {\color{blue}\(\triangleright\) Constant detrending}
        \State $\textsc{EMG} = \textsc{EMG} - \Call{Mean}{\textsc{EMG}, \textsc{axis}}$
        \State {\color{blue}\(\triangleright\) 4th order Butterworth bandpass filter}
        \State $\textsc{sampling\_rate} = \Call{Len}{\textsc{EMG}} / (t[-1] - t[0])$
        \State $\textsc{low} = $ $(2 * \textsc{bandpass\_freq\_low}) / \textsc{sampling\_rate}$
        \State $\textsc{high} = $ $(2 * \textsc{bandpass\_freq\_high}) / \textsc{sampling\_rate}$
        \State $\textsc{EMG} = \Call{sos\_bp}{\textsc{EMG}, \textsc{order}, [\textsc{low}, \textsc{high}], \textsc{axis}}$
        \State {\color{blue}\(\triangleright\) RMS envelope filter}
        \State $\textsc{window} = $  [1/1000, ..., 1/1000] {\color{blue} \Comment{1000-length}}
        \State {\textbf{for} i $\gets$ $[0,4)$ \textbf{do}:}
            \State \hskip1em $\textsc{EMG[$i$]} = \sqrt{\Call{conv}{\textsc{EMG[$i$]}^2, \textsc{window}}}$
        \State {\color{blue}\(\triangleright\) 4th order Butterworth lowpass filter}
        \State $\textsc{low} = $ $(2 * \textsc{lowpass\_freq}) / \textsc{sampling\_rate}$
        \State $\textsc{EMG} = $ \Call{sos\_lp}{\textsc{EMG}, \textsc{order}, \textsc{low}, \textsc{axis}}
        \State {\color{blue}\(\triangleright\) Left/Right normalization}
        \State $\textsc{EMG[0]} = \Call{max}{\textsc{EMG[1]}}/\Call{max}{\textsc{EMG[0]}}$ 
        \State $\textsc{EMG[2]} = \Call{max}{\textsc{EMG[3]}}/\Call{max}{\textsc{EMG[2]}}$ 
        \State {\color{blue}\(\triangleright\) Compute overall \activationShort}
        \State $\textsc{axis} = $ 1
        \State \textbf{return} $\Call{sum}{\textsc{EMG}, \textsc{axis}}$ {\color{blue} \Comment{Channel-wise sum}}
    \EndFunction
\end{algorithmic}
\end{tcolorbox}
\Caption{Our EMG data processing pipeline.}{The illustrated function filters and transforms multi-channel raw EMG signals into overall neck \activationShort.}
\label{fig:emg-processing-pseudo-code}
\end{figure}

%%%%%%%%%%%%%%%%%%%%%%%%%%%%%%%%%%%%%%%%%%%%%%%%%%%%%%%%%%%%%

\section{Implementation Details}
\label{supplementary:implementation}

\paragraph{EMG and head pose data collection and synchronization}
To collect EMG signals from both sides of sternocleidomastoid (SCM) and splenius capitis (SC) muscles, we employed 4 Delsys Trigno wireless EMG sensors synchronized at 2000 Hz. The captured 4-channel EMG signals were first wirelessly transmitted to a dedicated EMG base station, which then streamed the data to a Python program running on a desktop PC. To collect head pose data, we took advantage of the high-frequency (90 Hz) head tracking feature on Oculus Quest 2 head-mounted display (HMD). The tracked head pose data were transmitted to a Unity program running on the same desktop PC through Oculus Link. After the EMG data processing procedures described in \Cref{supplementary:emg-processing}, the two modalities were synchronized using system timestamps and re-sampled to 20 Hz.

\paragraph{Trajectory regression}
\TrajectoryNet takes in a pair of starting and ending head poses $\{\RotationStart \in \EuclideanThree,\RotationEnd \in \EuclideanThree\}$ and outputs the parameters of predicted Gaussian-shaped angular velocity curves for both pitch and yaw directions $\{\GaussianAmp^{i},\GaussianMean^{i},\GaussianStd^{i}\}_{i \in \{\Pitch,\Yaw\}}$. Specifically, $\{\RotationStart,\RotationEnd\}$ are first transformed into $\{\RotationStart,\RotationEnd-\RotationStart\}$ and then concatenated into a vector of length 4 before feeding into \TrajectoryNet for accelerated convergence during training and improved generalization ability of the model. To obtain the head motion trajectory $\Rotation_\TimeStamp(\RotationStart,\RotationEnd)$ associated with the predicted angular velocity $\AngularVelocity_\TimeStamp(\RotationStart,\RotationEnd)$, we integrate it over $[\TimeStampStart=0,\TimeStampEnd]$, where $\TimeStampEnd$ is determined such that:
\begin{align}
\RotationStart + \int_{\TimeStamp=0}^{\TimeStampEnd} \AngularVelocity_\TimeStamp(\RotationStart,\RotationEnd) \diff \TimeStamp = \RotationEnd.
\end{align}

\paragraph{\activationShort estimation}
The inputs to our \EnergyNet are composed of a head motion sequence of \TimeInterval=$400$ms, which is equivalent to 8 samples of pitch/yaw angles under the re-sampling rate of 20 Hz, and the corresponding angular acceleration values computed via finite difference (8 samples of pitch/yaw angular acceleration). Given the pair of input head motion and angular acceleration sequences (\TimeInterval=$400$ms, 8 samples for each), \EnergyNet outputs the instantaneous \activationShort for the central $200$ms interval (4 samples under the sampling rate of 20 Hz), i.e., compared to the outputs, the inputs cover additional $100$ms in both directions of the time axis.

\paragraph{\TrajectoryNet and \EnergyNet architectures}
\TrajectoryNet consists of 3 repeating FullyConnected-BatchNorm1D-ReLU blocks (the number of channels was set to 20, and the last block does not contain BatchNorm1D layer). The passive torque module $\PassiveTorque\left(\cdot\right)$ and torque-to-\activationShort module $\TorqueToEnergy\left(\cdot\right)$ of \EnergyNet were approximated by two 1D convolutional neural network (CNN) models. Specifically, $\PassiveTorque\left(\cdot\right)$ consists of 3 repeating Convolution1D-BatchNorm1D-ReLU blocks (number of channels was set to 20, and the last block does not contain ReLU activation); $\TorqueToEnergy\left(\cdot\right)$ consists of 3 repeating Convolution1D-BatchNorm1D-ReLU blocks (number of channels was set to 20), with the second one followed by a 1D MaxPooling layer (both kernel size and stride were set to 2) and the last one followed by a $20\times1$ FullyConnected layer.

\paragraph{\TrajectoryNet and \EnergyNet training}
\TrajectoryNet was optimized using $L_{2}$ loss and Adam optimizer ($\beta_{1}=0.9,\beta{2}=0.999$) for 25 epochs. The learning rate started at $1e^{-3}$ and dropped by $10\times$ at epoch 15. The batch size was set to 64. A weight decay factor of $1e^{-5}$ was enforced to reduce over-fitting. \EnergyNet was optimized using $L_{2}$ loss and Adam optimizer ($\beta_{1}=0.9,\beta{2}=0.999$) for 20 epochs. The learning rate started at $1e^{-3}$ and dropped by $10\times$ at epoch 10. The batch size was set to 64. A weight decay factor of $5e^{-4}$ was enforced to reduce over-fitting.

%%%%%%%%%%%%%%%%%%%%%%%%%%%%%%%%%%%%%%%%%%%%%%%%%%%%%%%%%%%%%

\section{Head Motion Statistics}
\label{supplementary:head-motion-statistics}

During both the pilot study (\Cref{sec:pilot}) and psychophysical study (\Cref{sec:results:study}), participants were instructed to move their heads as naturally as possible. No instruction or control on their head motion speed was given and participants were free to move faster or slower as they felt necessary. In our dataset, the maximum and mean velocities (degrees per second) for pitch/yaw are 182/238 and 94/133, while the maximum and mean accelerations (degrees per second squared) are 388/507 and 179/287.

%%%%%%%%%%%%%%%%%%%%%%%%%%%%%%%%%%%%%%%%%%%%%%%%%%%%%%%%%%%%%

\section{Generating User Study Conditions}
\label{supplementary:user-study-conditions}

\Cref{fig:user-study-conditions-pseudo-code} provides the implementation details of the condition generation algorithm in our psychophysical user study (\Cref{sec:results:study}).

\begin{figure}[ht]
\begin{tcolorbox}[
    enhanced,
    attach boxed title to top left={xshift=6mm,yshift=-3mm},
    colback=moonstoneblue!20,
    colframe=moonstoneblue,
    colbacktitle=moonstoneblue,
    title=User Study Condition Generation,
    fonttitle=\bfseries\color{black},
    boxed title style={size=small,colframe=moonstoneblue},
    sharp corners]
\medskip
\begin{algorithmic}[1]
    \Function{GetNextPose}{$\RotationStart$, $\TimeStamp$, $\theta^\circ$, \textsc{Condition}}
        \State {\color{blue}\(\triangleright\) Unif. sample 180 head poses that are $\theta^\circ$ from $\RotationStart$}
        \State $\textsc{poses} = \Call{UniformSample}{\RotationStart, \theta^\circ, 180}$
        \State $\textsc{all\_traj} = []$ 
        \State {\textbf{for} $\RotationEnd$ $\gets$ \textsc{poses} \textbf{do}:}
            \State \hskip1em {\color{blue}\(\triangleright\) Predict the head trajectory from $\RotationStart$ to $\RotationEnd$}
            \State \hskip1em $\textsc{trajectory} = \Call{\TrajectoryNet}{\RotationStart,\RotationEnd}$
            \State \hskip1em {\color{blue}\(\triangleright\) Include 1-second fixation on $\RotationEnd$}
            \State \hskip1em $\textsc{trajectory} = \Call{AddFixation}{\textsc{trajectory},\RotationEnd}$
            \State \hskip1em \textsc{all\_traj}.\Call{Append}{\textsc{trajectory}}
        \State {\color{blue}\(\triangleright\) Pick candidate with highest score as next pose}
        \State $\textsc{maxScore} = -\textsc{Inf}$
        \State \textsc{Init} $\PilotTargetPos$ {\color{blue} \Comment{Current candidate for next pose}}
        \State {\textbf{for} $i$ $\gets$ [0, ..., \Call{len}{\textsc{all\_traj}}-1] \textbf{do}:}
            \State \hskip1em $\RotationEnd = \Call{GetEndPose}{\textsc{all\_traj}[i]}$
            \State \hskip1em {\textbf{if} \textsc{Condition} == $\conditionMax$:}
                \State \hskip2em $\textsc{score} = \CoverageEnergy(\PilotTargetPos_{j\in[1,\TimeStamp]},\RotationEnd)+\CombinedEnergy(\textsc{all\_traj}[i])$
            \State \hskip1em {\textbf{if} \textsc{Condition} == $\conditionRand$:}
                \State \hskip2em $\textsc{score} = \CoverageEnergy(\PilotTargetPos_{j\in[1,\TimeStamp]},\RotationEnd)$
            \State \hskip1em {\textbf{if} \textsc{Condition} == $\conditionMin$:}
                \State \hskip2em $\textsc{score} = \CoverageEnergy(\PilotTargetPos_{j\in[1,\TimeStamp]},\RotationEnd)-\CombinedEnergy(\textsc{all\_traj}[i])$ 
            \State \hskip1em {\color{blue}\(\triangleright\) Update $\PilotTargetPos$ if $\textsc{score}$ greater than $\textsc{maxScore}$}
            \State \hskip1em {\textbf{if} $\textsc{score} > \textsc{maxScore}$:}
                \State \hskip2em $\textsc{maxScore} = \textsc{Score}$
                \State \hskip2em $\PilotTargetPos = \RotationEnd$
        \State \textbf{return} $\PilotTargetPos$
    \EndFunction
\end{algorithmic}
\end{tcolorbox}
\Caption{User study condition generation algorithm.}{Given the current head pose $\RotationEnd$ on a scan path, this function extends the scan path by generating the optimal next head pose $\PilotTargetPos$ for one of the 3 conditions $\conditionMax$/$\conditionMin$/$\conditionRand$.}
\label{fig:user-study-conditions-pseudo-code}
\end{figure}

%%%%%%%%%%%%%%%%%%%%%%%%%%%%%%%%%%%%%%%%%%%%%%%%%%%%%%%%%%%%%

\section{Individual Votes in User Study}
\label{supplementary:user-study-votes}

\Cref{tab:user-study} summarizes all 12 user study (\Cref{sec:results:study}) participants' two-alternative forced choice (2AFC) response distribution across the three conditions: $\conditionMax$, $\conditionRand$, and $\conditionMin$. Each number indicates the number of times that a particular condition was chosen as the more uncomfortable one over all 18 2AFC sessions.

\begin{table}[!hbp]
\begin{adjustbox}{max width=0.48\textwidth}
  \centering
  \tabtextsize
  \begin{tabular}{|l|c|c|c|c|c|c|c|c|c|c|c|c|}
    \hline
    \diagbox{cond}{user} & \#1 & \#2 & \#3 & \#4 & \#5 & \#6 & \#7 & \#8 & \#9 & \#10 & \#11 & \#12\\
    \hline
    $\conditionMax$& 11 & 12 & 11 & 12 & 10 & 10 & 9 & 12 & 9 & 10 & 9 & 9\\
    \hline
    $\conditionRand$& 5 & 5 & 6 & 4 & 4 & 7 & 8 & 6 & 7 & 6 & 6 & 9\\
    \hline
    $\conditionMin$& 2 & 1 & 1 & 2 & 4 & 1 & 1 & 0 & 2 & 2 & 3 & 0\\
    \hline
  \end{tabular}
  \end{adjustbox}
  \Caption{Individual 2AFC results in user study.}{The numbers indicate, for each participant and each condition, how many trials among all 18 2AFC sessions that particular condition was rated by that particular participant as being more uncomfortable.}
  \label{tab:user-study}
\end{table}
