# Supplementary material for: Toward Optimized VR/AR Ergonomics: Modeling and Predicting User Neck Muscle Contraction
Source: arXiv:2308.14841 source file (2023-08-28)
Supplement: Supplementary file 2 [file supplementary_emg_processing.tex]

\begin{figure}[h!]
\begin{tcolorbox}[
    enhanced,
    attach boxed title to top left={xshift=6mm,yshift=-3mm},
    colback=moonstoneblue!20,
    colframe=moonstoneblue,
    colbacktitle=moonstoneblue,
    title=EMG to \activationShort Data Processing Pipeline,
    fonttitle=\bfseries\color{black},
    boxed title style={size=small,colframe=moonstoneblue},
    sharp corners]
\medskip
\begin{algorithmic}[1]
    \Function{EMG2\activationShort}{EMG}
        \State {\color{blue}\(\triangleright\) 4-channel EMG signals}
        \State $t = \Call{GetTimestamps}{\textsc{EMG}}$ {\color{blue} \Comment{EMG timestamps}}
        \State $\textsc{axis} = $ 0
        \State $\textsc{bandpass\_freq\_low} = $ 20 Hz
        \State $\textsc{bandpass\_freq\_high} = $ 150 Hz
        \State $\textsc{lowpass\_freq} = $ 1 Hz
        \State $\textsc{butterworth\_order} = $ 4
        \State {\color{blue}\(\triangleright\) Constant detrending}
        \State $\textsc{EMG} = \textsc{EMG} - \Call{Mean}{\textsc{EMG}, \textsc{axis}}$
        \State {\color{blue}\(\triangleright\) 4th order Butterworth bandpass filter}
        \State $\textsc{sampling\_rate} = \Call{Len}{\textsc{EMG}} / (t[-1] - t[0])$
        \State $\textsc{low} = $ $(2 * \textsc{bandpass\_freq\_low}) / \textsc{sampling\_rate}$
        \State $\textsc{high} = $ $(2 * \textsc{bandpass\_freq\_high}) / \textsc{sampling\_rate}$
        \State $\textsc{EMG} = \Call{sos\_bp}{\textsc{EMG}, \textsc{order}, [\textsc{low}, \textsc{high}], \textsc{axis}}$
        \State {\color{blue}\(\triangleright\) RMS envelope filter}
        \State $\textsc{window} = $  [1/1000, ..., 1/1000] {\color{blue} \Comment{1000-length}}
        \State {\textbf{for} i $\gets$ $[0,4)$ \textbf{do}:}
            \State \hskip1em $\textsc{EMG[$i$]} = \sqrt{\Call{conv}{\textsc{EMG[$i$]}^2, \textsc{window}}}$
        \State {\color{blue}\(\triangleright\) 4th order Butterworth lowpass filter}
        \State $\textsc{low} = $ $(2 * \textsc{lowpass\_freq}) / \textsc{sampling\_rate}$
        \State $\textsc{EMG} = $ \Call{sos\_lp}{\textsc{EMG}, \textsc{order}, \textsc{low}, \textsc{axis}}
        \State {\color{blue}\(\triangleright\) Left/Right normalization}
        \State $\textsc{EMG[0]} = \Call{max}{\textsc{EMG[1]}}/\Call{max}{\textsc{EMG[0]}}$ 
        \State $\textsc{EMG[2]} = \Call{max}{\textsc{EMG[3]}}/\Call{max}{\textsc{EMG[2]}}$ 
        \State {\color{blue}\(\triangleright\) Compute overall \activationShort}
        \State $\textsc{axis} = $ 1
        \State \textbf{return} $\Call{sum}{\textsc{EMG}, \textsc{axis}}$ {\color{blue} \Comment{Channel-wise sum}}
    \EndFunction
\end{algorithmic}
\end{tcolorbox}
\Caption{Our EMG data processing pipeline.}{The illustrated function filters and transforms multi-channel raw EMG signals into overall neck \activationShort.}
\label{fig:emg-processing-pseudo-code}
\end{figure}
