# Supplementary material for: Toward Optimized VR/AR Ergonomics: Modeling and Predicting User Neck Muscle Contraction
Source: arXiv:2308.14841 source file (2023-08-28)
Supplement: Supplementary file 3 [file supplementary_user_study_conditions.tex]

\begin{figure}[ht]
\begin{tcolorbox}[
    enhanced,
    attach boxed title to top left={xshift=6mm,yshift=-3mm},
    colback=moonstoneblue!20,
    colframe=moonstoneblue,
    colbacktitle=moonstoneblue,
    title=User Study Condition Generation,
    fonttitle=\bfseries\color{black},
    boxed title style={size=small,colframe=moonstoneblue},
    sharp corners]
\medskip
\begin{algorithmic}[1]
    \Function{GetNextPose}{$\RotationStart$, $\TimeStamp$, $\theta^\circ$, \textsc{Condition}}
        \State {\color{blue}\(\triangleright\) Unif. sample 180 head poses that are $\theta^\circ$ from $\RotationStart$}
        \State $\textsc{poses} = \Call{UniformSample}{\RotationStart, \theta^\circ, 180}$
        \State $\textsc{all\_traj} = []$ 
        \State {\textbf{for} $\RotationEnd$ $\gets$ \textsc{poses} \textbf{do}:}
            \State \hskip1em {\color{blue}\(\triangleright\) Predict the head trajectory from $\RotationStart$ to $\RotationEnd$}
            \State \hskip1em $\textsc{trajectory} = \Call{\TrajectoryNet}{\RotationStart,\RotationEnd}$
            \State \hskip1em {\color{blue}\(\triangleright\) Include 1-second fixation on $\RotationEnd$}
            \State \hskip1em $\textsc{trajectory} = \Call{AddFixation}{\textsc{trajectory},\RotationEnd}$
            \State \hskip1em \textsc{all\_traj}.\Call{Append}{\textsc{trajectory}}
        \State {\color{blue}\(\triangleright\) Pick candidate with highest score as next pose}
        \State $\textsc{maxScore} = -\textsc{Inf}$
        \State \textsc{Init} $\PilotTargetPos$ {\color{blue} \Comment{Current candidate for next pose}}
        \State {\textbf{for} $i$ $\gets$ [0, ..., \Call{len}{\textsc{all\_traj}}-1] \textbf{do}:}
            \State \hskip1em $\RotationEnd = \Call{GetEndPose}{\textsc{all\_traj}[i]}$
            \State \hskip1em {\textbf{if} \textsc{Condition} == $\conditionMax$:}
                \State \hskip2em $\textsc{score} = \CoverageEnergy(\PilotTargetPos_{j\in[1,\TimeStamp]},\RotationEnd)+\CombinedEnergy(\textsc{all\_traj}[i])$
            \State \hskip1em {\textbf{if} \textsc{Condition} == $\conditionRand$:}
                \State \hskip2em $\textsc{score} = \CoverageEnergy(\PilotTargetPos_{j\in[1,\TimeStamp]},\RotationEnd)$
            \State \hskip1em {\textbf{if} \textsc{Condition} == $\conditionMin$:}
                \State \hskip2em $\textsc{score} = \CoverageEnergy(\PilotTargetPos_{j\in[1,\TimeStamp]},\RotationEnd)-\CombinedEnergy(\textsc{all\_traj}[i])$ 
            \State \hskip1em {\color{blue}\(\triangleright\) Update $\PilotTargetPos$ if $\textsc{score}$ greater than $\textsc{maxScore}$}
            \State \hskip1em {\textbf{if} $\textsc{score} > \textsc{maxScore}$:}
                \State \hskip2em $\textsc{maxScore} = \textsc{Score}$
                \State \hskip2em $\PilotTargetPos = \RotationEnd$
        \State \textbf{return} $\PilotTargetPos$
    \EndFunction
\end{algorithmic}
\end{tcolorbox}
\Caption{User study condition generation algorithm.}{Given the current head pose $\RotationEnd$ on a scan path, this function extends the scan path by generating the optimal next head pose $\PilotTargetPos$ for one of the 3 conditions $\conditionMax$/$\conditionMin$/$\conditionRand$.}
\label{fig:user-study-conditions-pseudo-code}
\end{figure}
